# Supplementary material for: Soft Rasterizer: Differentiable Rendering for Unsupervised Single-View Mesh Reconstruction
Source: arXiv:1901.05567 source file (2019-01-23)
Supplement: Supplementary file 1 [file fig_supple_deform_process.tex]

\begin{figure*}[h]
    \vspace{-10px}
        \includegraphics[width=1.0\linewidth]{supple_deform_process_v1.pdf}
    \vspace{-5px}
    \caption{Demonstration for mesh deformation process while training on only one input image.}
    \label{fig:supple_deform_process}
\end{figure*}
