# Supplementary material for: Soft Rasterizer: Differentiable Rendering for Unsupervised Single-View Mesh Reconstruction
Source: arXiv:1901.05567 source file (2019-01-23)
Supplement: Supplementary file 2 [file fig_supple_more_result.tex]

\begin{figure*}[t!]
    \vspace{-10px}
    \includegraphics[scale=0.4]{supple_more_result_part_1_v1.png}
    \centering
    \vspace{-5px}
    \caption{More reconstruction results using our approach. Leftmost column: input image; the rest columns: results visualized from multiple viewpoints.}
    \label{fig:supple_more_result_part_1}
\end{figure*}

\begin{figure*}[t!]
    \vspace{-10px}
    \includegraphics[scale=0.4]{supple_more_result_part_2_v1.png}
    \centering
    \vspace{-5px}
    \caption{More reconstruction results using our approach. Leftmost column: input image; the rest columns: results visualized from multiple viewpoints.}
    \label{fig:supple_more_result_part_2}
\end{figure*}

\begin{figure*}[t!]
    \vspace{-10px}
    \includegraphics[scale=0.4]{supple_more_result_part_3_v1.png}
    \centering
    \vspace{-5px}
    \caption{More reconstruction results using our approach. Leftmost column: input image; the rest columns: results visualized from multiple viewpoints.}
    \label{fig:supple_more_result_part_3}
\end{figure*}
